# Supplementary material for: disco: a toolkit for Distributional Control of Generative Models
Source: arXiv:2303.05431 source file (2023-03-08)
Supplement: Supplementary file 1 [file appendix.tex]

\appendix
\clearpage
\section{Appendix}

\subsection{Experiments}

\subsubsection{Amazing Experiment}

\begin{pythoncode*}{fontsize=\scriptsize}
prefix, word = "", "amazing"
n_steps, n_samples_per_step = 1000, 2*2**10
sampling_size, scoring_size = 2**6, 2**6

single_word_scorer = BooleanScorer(
        lambda s, _: word in s.text
    )

base = LMDistribution(device=0)
target = base.constrain(
        [single_word_scorer], [1]
    )

model = LMDistribution(
        freeze=False, device=0
    )

features = [
        (word, single_word_scorer)
    ]

tuner = DPGTuner(model, target,
    context=prefix,
    features=features, 
    n_gradient_steps=n_steps,
    n_samples_per_step=n_samples_per_step,
    sampling_size=sampling_size,
    scoring_size=scoring_size)

console = ConsoleLogger(tuner)

tuner.tune()

stamp = datetime.now()\
    .strftime("%Y_%m_%d-%H:%M")
torch.save(model,
    f"{<PATH>}/{word}.{stamp}.pt")

\end{pythoncode*}

\subsubsection{Don't Hallucinate Entities}

\begin{pythoncode*}{fontsize=\scriptsize}
nlp = spacy.load("en_core_web_sm")

def entities(text,
        types=["GPE", "PERSON", "ORG"]):
    """set of entities in text"""
    doc = nlp(text)
    return set(
        e.text\
            .lower().strip()\
            .split('.<')[0]\
        for e in doc.ents\
            if e.label_ in types)

no_new_entity_scorer = BooleanScorer(
        lambda s, c: all({
                any(es in ec for ec in entities(c))\
                    for es in entities(s.text)
            })
    )
at_least_two_entities_scorer = BooleanScorer(
        lambda s, _: 1 <= len(entities(s.text))
    )

t5 = "t5-small"
base = LMDistribution(
        network=t5, tokenizer=t5,
        nature="seq2seq", device=0
    )

target = base\
        * no_new_entity_scorer\
        * at_least_two_entities_scorer

model = LMDistribution(
        network=t5, tokenizer=t5,
        nature="seq2seq", device=0,
        length=256, freeze=False)

features = [
        ("no new ent",
            no_new_entity_scorer),
        ("at least 2 ents",
            at_least_two_entities_scorer)
    ]

contexts = DatasetContextDistribution(
        dataset="cnn_dailymail",
        subset="1.0.0",
        split="train[:5000]",
        key="article",
        prefix="summarize: "
    )

tuner = CDPGTuner(model, target,
        context_distribution=contexts,
        features=features,
        n_gradient_steps=1000,
        n_samples_per_step=2*2**10,
        context_sampling_size=2**3,
        sampling_size=2**8,
        scoring_size=2**8)

wandb = WandBLogger(
    tuner,
    project="disco"
)

tuner.tune()

stamp = datetime.now()\
    .strftime("%Y_%m_%d-%H:%M")
torch.save(model,
    f"{<PATH>}/entities.{stamp}.pt")
\end{pythoncode*}

\subsubsection{The Entertainer}

\begin{pythoncode*}{fontsize=\scriptsize}
def myers_briggs(input_text):
    """seee appendix for body"""
    
    return {
            "I": round(i, 2), "E": round(e, 2),
            "N": round(n, 2), "S": round(s, 2),
            "T": round(t, 2), "F": round(f, 2),
            "J": round(j, 2), "P": round(p, 2)
        }

class PersonalityTypeScorer(PositiveScorer):

    def __init__(self, personality, separator, eos):
        """
        Parameters
        ----------
        personality: string
            personality expected in a text
        separator: char
            expected separator between utterances
        eos: char
            end of sequence character
        """

        super(PersonalityTypeScorer, self)\
            .__init__(lambda s, _: myers_briggs(
                (s.text.replace('<s>', '', 1)\
                    if s.text.startswith('<s>')\
                    else s.text)\
                .split(separator)[0])[personality]
            )

blender = "facebook/blenderbot-400M-distill"
base = LMDistribution(
        network=blender,
        tokenizer=blender,
        nature="seq2seq",
        device=0
    )

sep, eos = '<s>', '</s>'
contexts = ContextDistribution(
            "data/icebreakers.txt")

pts_E = PersonalityTypeScorer("E", sep, eos)
pts_S = PersonalityTypeScorer("S", sep, eos)
pts_F = PersonalityTypeScorer("F", sep, eos)
pts_P = PersonalityTypeScorer("P", sep, eos)
target = base.constrain(
    [pts_E, pts_S, pts_F, pts_P],
    [0.8] * 4,
    context_distribution=contexts,
    context_sampling_size=2**4, n_samples=2**8
)

model = LMDistribution(
        network=blender,
        tokenizer=blender,
        nature="seq2seq", length=60,
        freeze=False, device=0
    )

features = [
        ("E", pts_E,
        ("S", pts_S,
        ("F", pts_F,
        ("P", pts_P,
    ]

contexts = ContextDistribution(
        "data/icebreakers.txt"
    )

tuner = CDPGTuner(model, target,
    context=contexts,
    features = features,
    n_gradient_steps=2000,
    n_samples_per_step=512,
    context_sampling_size=8,
    sampling_size=128,
    scoring_size=128)

neptune = NeptuneLogger(
    tuner,
    project="disco", api_token=<TOKEN>
)

tuner.tune()

stamp = datetime.now()\
    .strftime("%Y_%m_%d-%H:%M")
torch.save(model,
    f"{SAVE_PATH}/esfp.{stamp}.pt")
 
\end{pythoncode*}
